# Supplementary material for: Emergent organization of receptive fields in networks of excitatory and inhibitory neurons
Source: arXiv:2205.13614 source file (2022-05-26)
Supplement: Supplementary file 1 [file additional.tex]

% !TEX root = surfing.tex

\section{Additional Simulations}
\label{sec:addsims}

Here we give additional plots for experiments comparing surfing over a sequence of networks during training to gradient descent over the final trained network. As described in the main text,
we consider the problem of minimizing the objective $f(x) = \frac{1}{2}\|G(x) - G(x_*)\|^2$, that is, recovering the image generated from a trained network $G(x) = G_{\theta_T}(x)$ with input $x_*$. We run surfing by taking a sequence of parameters $\theta_0, \theta_1,...,\theta_T$, where $\theta_0$ are the initial random parameters and the intermediate $\theta_t$'s are taken every 40 training steps. In order to improve convergence speed we use Adam \citep{kingma2014adam} to carry out gradient descent in each step in surfing. We also use Adam when optimizing over the just the final network. We apply surfing and regular Adam for 300 trials, where in each trial a randomly generated $x_*$ and initial point $x_{init}$ is chosen. Figure \ref{fig:more} shows
the distribution of the distance between the computed solution $\hat x_T$ and the truth $x_*$ for VAE, WGAN and WGAN-GP,
using surfing (red) and regular gradient descent with Adam (blue), over three different input dimensions $k$.

\begin{figure}[h]
\begin{center}
\begin{tabular}{ccc}
  \\[20pt]
\includegraphics[width=.3\textwidth]{newfigs/VAEdim-5} &
\includegraphics[width=.3\textwidth]{newfigs/VAEdim-10} &
\includegraphics[width=.3\textwidth]{newfigs/VAEdim-20} \\
\includegraphics[width=.3\textwidth]{newfigs/WGANdim-5} &
\includegraphics[width=.3\textwidth]{newfigs/WGANdim-10} &
\includegraphics[width=.3\textwidth]{newfigs/WGANdim-20}\\
\includegraphics[width=.3\textwidth]{newfigs/WGAN-GPdim-5} &
\includegraphics[width=.3\textwidth]{newfigs/WGAN-GPdim-10} &
\includegraphics[width=.3\textwidth]{newfigs/WGAN-GPdim-20}
\end{tabular}
\end{center}
\caption{Distribution of the distance between solution $\hat x_T$ and the truth $x_*$ for VAE, WGAN and WGAN-GP,
using surfing (red) and regular gradient descent with Adam (blue) over three different input dimensions $k$.}
\label{fig:more}
\end{figure}
